# Supplementary material for: Probabilistic Implicit Scene Completion
Source: arXiv:2204.01264 source file (2022-04-04)
Supplement: Supplementary file 1 [file appendix_neurips.tex]

\section{Proofs and Derivations of Maximizing Variational Lower Bound}
\label{appendix:proofs_and_derivations}
\subsection{Proof of Proposition 1} \label{appendix:prop1}
Recall the proposition~\ref{prop:infusion_convergence}.
\infusionconvergence*
\begin{proof}
	Since $\alpha^t$ is increasing, there exists $T_0$ such that $\alpha^{T_0} = 1$.
	Then the infusion transition kernel $q$ becomes a deterministic function with next state defined by $s^{t + 1} = G_x(s^t),\; \forall t \ge T_0$.
	We now prove that the sequence $s^{t + 1} = G_x(s^t)$ converges to $x$ in a finite number of steps.
	x
	We first find $T_1$ such that $x \subset s^{T_0 + T_1}$ for $t \ge T_0 + T_1$.
	Let $c \in x$.
	We define a sequence of coordinates $c_t = argmin_{c' \in s^{T_0 +t}} d(c, c')$ and sequence of distances $d_t = \min_{c' \in s^{T_0 +t}}$, $d(c, c')$.
	Since $s^{t + 1} = G_x(s^t) = \{\mathrm{argmin}_{c \in \mathcal{N}(s^t)}  d(c, c') \mid c' \in x\}$ and $s^t \subsetneq \mathcal{N}(s^t)$, $d_t$ is a decreasing function bounded by $0$.
	Thus, there exists $T_1$ such that $d_{T_1} = 0$, which implies that corresponding coordinate $c_{T_1} = c$.
	
	Now, consider a state $s^{T_0 + T_1 + 1} = G_x(s^{T_0 + T_1}) = \{\mathrm{argmin}_{c \in \mathcal{N}(s^{T_0 + T_1})}  d(c, c') \mid c' \in x\}$.
	$x \subset s^{T_0 + T_1} \subset \mathcal{N}(s^{T_0 + T_1})$.
	This implies $\min_{c \in \mathcal{N}(s^{T_0 + T_1})} d(c, c') = 0$ for all $c' \in x$. 
	Thus, $x = s^{T_0 + T_1 + 1}$.
	Setting $T = T_0 + T_1 + 1$ concludes the proof.x
\end{proof}
\vspace{-1em}

\subsection{Detailed Derivation of Eq~\ref{eq:elbo}}
\label{section:detailed_derivation}
\begin{align*}
	\log p_\theta (s^T)
	&= \log \sum_{s^{0:T - 1}} p_\theta (s^{0:T}) \\
	&= \log \sum_{s^{0:T - 1}} q_\phi (s^{0:T-1} | s^T) \frac{p_\theta (s^{0:T})}{q_\phi (s^{0:T-1} | s^T)} \\
	&\ge \sum_{s^{0:T - 1}} q_\phi (s^{0:T-1} | s^T)  \log \frac{p_\theta (s^{0:T})}{q_\phi (s^{0:T-1} | s^T)} \quad (\because \text{Jensen's inequality}) \\
	&= \sum_{s^{0:T - 1}} q_\phi (s^{0:T-1} | s^T) (
		\log \frac{p (s^0)}{q (s^0)}
		+ \log p (s^T | s^{T -1 })
		+ \sum_{0 \leq t < T - 1} \log \frac{p_\theta (s^{t + 1}|s^t)}{q_\phi (s^{t + 1}|s^t, s^T)}
	)
\end{align*}
The third term of right hand side can be converted into KL divergence as following: 
\begin{align*}
	&\sum_{s^{0:T - 1}} q_\phi (s^{0:T-1} | s^T) \sum_{0 \leq t < T - 1} \log \frac{p_\theta (s^{t + 1}|s^t)}{q_\phi (s^{t + 1}|s^t, s^T)} \\
	&= \sum_{s^{0:T - 1}} \prod_{0 \leq i < T - 1} q_\phi (s^{i + 1} |s^i, s^T) \sum_{0 \leq t < T - 1} \log \frac{p_\theta (s^{t + 1}|s^t)}{q_\phi (s^{t + 1}|s^t, s^T)} \\
	&= \sum_{s^{0:T - 1}} \sum_{0 \leq t < T - 1} \prod_{\substack{0 \leq i < T - 1 \\ i\neq t}} q_\phi (s^{i + 1} |s^i, s^T) q_\phi (s^{t + 1} |s^t, s^T) \log \frac{p_\theta (s^{t + 1}|s^t)}{q_\phi (s^{t + 1}|s^t, s^T)} \\
	&= \sum_{0 \leq t < T - 1} \sum_{s^{t + 1}} (
		\sum_{s^{-(t + 1)}}
		\prod_{\substack{0 \leq i < T - 1 \\ i\neq t}} q_\phi (s^{i + 1} |s^i, s^T)
	)
	q_\phi (s^{t + 1} |s^t, s^T) \log \frac{p_\theta (s^{t + 1}|s^t)}{q_\phi (s^{t + 1}|s^t, s^T)} \\
	& \quad (s^{-(t + 1)} \text{ denotes variables $s^{0:T - 1}$ except } s^{t + 1})\\
	&= \sum_{0 \leq t < T - 1} \sum_{s^{t + 1}}
	q_\phi (s^{t + 1} |s^t, s^T) \log \frac{p_\theta (s^{t + 1}|s^t)}{q_\phi (s^{t + 1}|s^t, s^T)}\\
	&= -\sum_{0 \leq t < T - 1} \sum_{s^{t + 1}}
	q_\phi (s^{t + 1} |s^t, s^T) \log \frac{q_\phi (s^{t + 1}|s^t, s^T)}{p_\theta (s^{t + 1}|s^t)}\\
	&= -\sum_{0 \leq t < T - 1} D_{KL}(q_\phi (s^{t + 1}|s^t, s^T) || p_\theta (s^{t + 1}|s^t))
\end{align*}
Thus,
\begin{equation*}
	\log p_\theta(s^T) = \log \frac{p(s^0)}{q(s^0)} + \E_{q_\phi}[\log p_\theta(s^T | s^{T - 1})] - \sum_{0 \le t < T - 1} D_{KL}(q_\phi(s^{t + 1} | s^t, s^T) || p_\theta(s^{t + 1} | s^t))) 
\end{equation*}
is derived.
\subsection{Proof of Proposition 2} \label{appendix:prop2}
Recall the proposition~\ref{prop:maximizing_lower_bound}.

\maximizinglowerbound*

We first show a lemma that the KL divergence of factorized distribution can be decomposed as 
sum of factorization.
\begin{lemma} \label{lemma:kl_factorization}
	Suppose the two distribution $q, p$ can be factorized as following:
	\begin{align*}
		q(z_1, z_2, ..., z_N) = \prod_{0 \le i \le N} q(z_i) \\
		p(z_1, z_2, ..., z_N) = \prod_{0 \le i \le N} p(z_i)
	\end{align*}
	Then, 
	\begin{equation*}
		D_{KL} (q(z_1, z_2, ..., z_N) || p(z_1, z_2, ..., z_N)) = \sum_{0 \le i \le N} D_{KL} (q(z_i) || p(z_i))
	\end{equation*}
	
	\begin{proof}
		We first show the case where there are $N=2$ variables.
		\begin{align*}
		D_{KL}(q(z_1, z_2) || p(z_1, z_2))) 
		&=\sum_{z_1, z_2} q(z_1, z_2) \log \frac{q(z_1, z_2)}{p(z_1, z_2)} \\
		&=\sum_{z_1, z_2} q(z_1)q( z_2) \log \frac{q(z_1) q(z_2)}{p(z_1) p(z_2)} \\
		&=\sum_{z_1, z_2} q(z_1)q( z_2) ( \log \frac{q(z_1)}{p(z_1)} + \log \frac{q(z_2)}{p(z_2)}) \\
		&=\sum_{z_1, z_2} q(z_1)q( z_2) \log \frac{q(z_1)}{p(z_1)} + \sum_{z_1, z_2} q(z_1)q( z_2) \log \frac{q(z_2)}{p(z_2)} \\
		&=  \sum_{z_1} q(z_1)  \log \frac{q(z_1)}{p(z_1)} (\sum_{z_2} q( z_2)) 
		+ \sum_{z_2}q( z_2) \log \frac{q(z_2)}{p(z_2)} (\sum_{z_1} q( z_1)) \\
		&=\sum_{z_1} q(z_1)  \log \frac{q(z_1)}{p(z_1)} + \sum_{z_2}q( z_2) \log \frac{q(z_2)}{p(z_2)} \\
		&=	D_{KL} (q(z_1) || p(z_1)) + D_{KL} (q(z_2) || p(z_2))
		\end{align*}
		Using the above $N$ times iteratively by decomposing single variable at a time provides a direct proof for $N \ge 2$ case.
	\end{proof}
\end{lemma}

\begin{proof}
	We first factorize the KL divergence of state into cells and apply the definition of $q$ distribution.
	\begin{align*}
	D_{KL}(q_\theta(s^{t + 1} | s^t, s^T) || p_\theta(s^{t + 1} | s^t))
	&=  \sum_ {c \in s^{t + 1}}D_{KL}(q_\theta(c | s^t, s^T) || p_\theta(c| s^t)) \quad(\because \text{Lemma~\ref{lemma:kl_factorization}}) \\
	&= \sum_ {c \in s^{t + 1}} q_\theta(c | s^t, s^T) \log \frac{q_\theta(c | s^t, s^T)}{p_\theta(c | s^t)} \\
	&= \sum_ {c \in s^{t + 1}} ((1 - \alpha^t)p_\theta(c | s^t)  + \alpha^t \delta_{G_x(s^t)}(c)) \log \frac{(1 - \alpha^t)p_\theta(c | s^t)  + \alpha^t \delta_{G_x(s^t)}(c)}{p_\theta(c | s^t)} \\
	&= \sum_ {c \in s^{t + 1}} h_{s^t}(p_\theta(c | s^t))
	\end{align*}
	
	where $h_{s^t}$ is defined as
	\begin{equation*}
		h_{s^t}(\mu) = ((1 - \alpha^t)\mu  + \alpha^t \delta_{G_x(s^t)}(c)) \log \frac{(1 - \alpha^t)\mu  + \alpha^t \delta_{G_x(s^t)}(c)} {\mu}.
	\end{equation*}
	We now show that $h_{s^t}(\mu)$ is a decreasing function with respect to $\mu$.
	The cases are divided whether $\delta_{G_x(s^t)}(c) = 0$ or $\delta_{G_x(s^t)}(c) = 1$.
	
	If $\delta_{G_x(s^t)}(c) = 0$,
	\begin{equation*}
		h_{s^t}(\mu) 	= (1 - \alpha^t) \mu \log (1 - \alpha^t) \\
	\end{equation*}
	\begin{align*}
	\frac{d}{d\mu}h_{s^t}(\mu) 
	&= (1 - \alpha^t) \log (1 - \alpha^t) \\
	&\leq 0 \quad (\because 0 < \alpha^t < 1)
	\end{align*}
	
	If $\delta_{G_x(s^t)}(c) = 1$,
	\begin{equation}
		h_{s^t}(\mu) = ((1 - \alpha^t)\mu  + \alpha^t ) \log \frac{(1 - \alpha^t)\mu  + \alpha^t} {\mu}
	\end{equation}
	\begin{align*}
	\frac{d}{d\mu}h_{s^t}(\mu) 
	&= (1 - \alpha^t) \log (1 - \alpha^t + \frac{\alpha^t}{\mu}) - \frac{1}{\mu} \\
	&= (1 - \alpha^t) (\log (1 - \alpha^t ) + \log (1 + \frac{\alpha^t}{(1 - \alpha^ t)\mu})) - \frac{1}{\mu} \\
	&\leq (1 - \alpha^t) \log (1 - \alpha^t ) + \frac{\alpha^t}{\mu} - \frac{1}{\mu} \quad (\because \log (1 + x) \leq x, \; \forall x > 0) \\
	&\leq (1 - \alpha^t) (\log (1 - \alpha^t ) - \frac{1}{\mu}) \\
	&\leq 0 \quad (\because 0 < \alpha^t < 1)
	\end{align*}
	Thus, $h_{s^t}$ is a decreasing function concluding that $D_{KL}(q_\theta(s^{t + 1} | s^t, s^T) || p_\theta(s^{t + 1} | s^t)) \le D_{KL}(q_{\theta'}(s^{t + 1} | s^t, s^T) || p_{\theta'}(s^{t + 1} | s^t))$  for $ p_{\theta'}(c | s^t) \ge p_{\theta}(c | s^t), \; \forall c \in s^{t+1}$.
\end{proof}

\section{Comparison with GCA}
\label{appendix:gca_comparison}
We emphasize the stochastic voxel generation loss in cGCA models 1) theoretically valid loss while GCA does not, 2) can generate any shapes without connetivity assumption.

\section{Effects of Mode Seeking Steps}
\label{appendix:mode_seeking_steps}

\section{Implementation Details}
\label{appendix:implementation_details}

\subsection{Neural Network Architecture and Implementation Details}
\todo{checklist: hyperparameter}

\todo{checklist: computing resources}
\subsection{Data Preparation}
\label{appendix:data_preparation}
\todo{checklist: data split, both}\\
\textbf{ShapeNet.} \todo{include data splits, how they are chosen}

\textbf{3DFront.} \todo{include data splits, how they are chosen}

\label{appendix:baselines}
\subsection{Baselines}
\textbf{GCA~\cite{zhang2021gca}.} \todo{include hyperparameters}

\textbf{NDF~\cite{chibane2020ndf}.} \todo{include hyperparameters}

\subsection{Evaluation Metrics}
